# Supplementary material for: LooC: Effective Low-Dimensional Codebook for Compositional Vector Quantization
Source: arXiv:2601.00222 source file (2026-01-01)
Supplement: Supplementary file 1 [file supp_generation.tex]

\begin{figure*}[t]
  \centering
   %\fbox{\rule{0pt}{2in} \rule{0.9\linewidth}{0pt}}
   \includegraphics[width=0.98\linewidth]{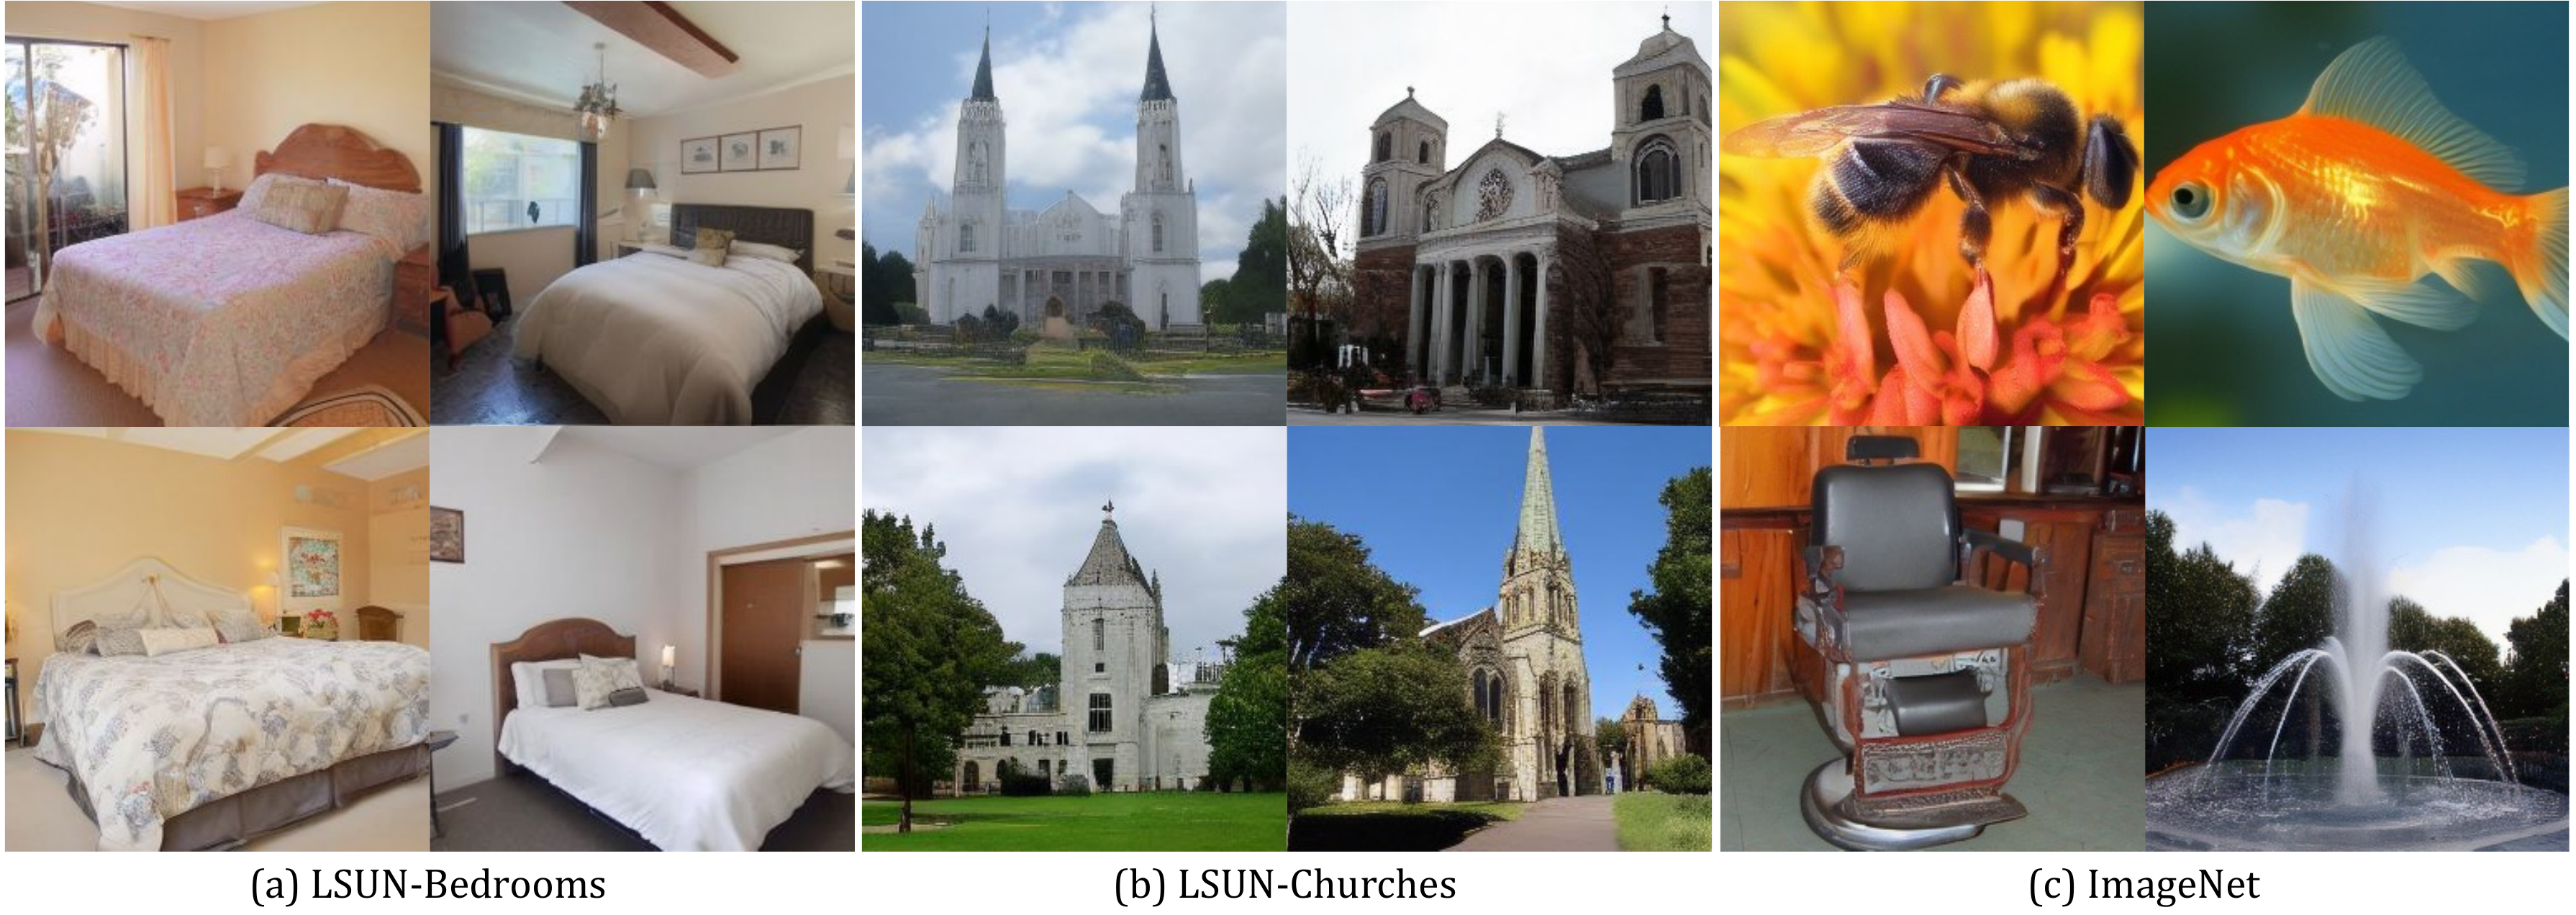}

   \caption{ Unconditional image generation on LSUN, and class-conditional image generation on Imagenet.
    }
   \label{supp_fig_generation}
\end{figure*}
