# Supplementary material for: LooC: Effective Low-Dimensional Codebook for Compositional Vector Quantization
Source: arXiv:2601.00222 source file (2026-01-01)
Supplement: Supplementary file 2 [file supp_reconstruction.tex]

\begin{figure*}[t]
  \centering
   %\fbox{\rule{0pt}{2in} \rule{0.9\linewidth}{0pt}}
   \includegraphics[width=0.98\linewidth]{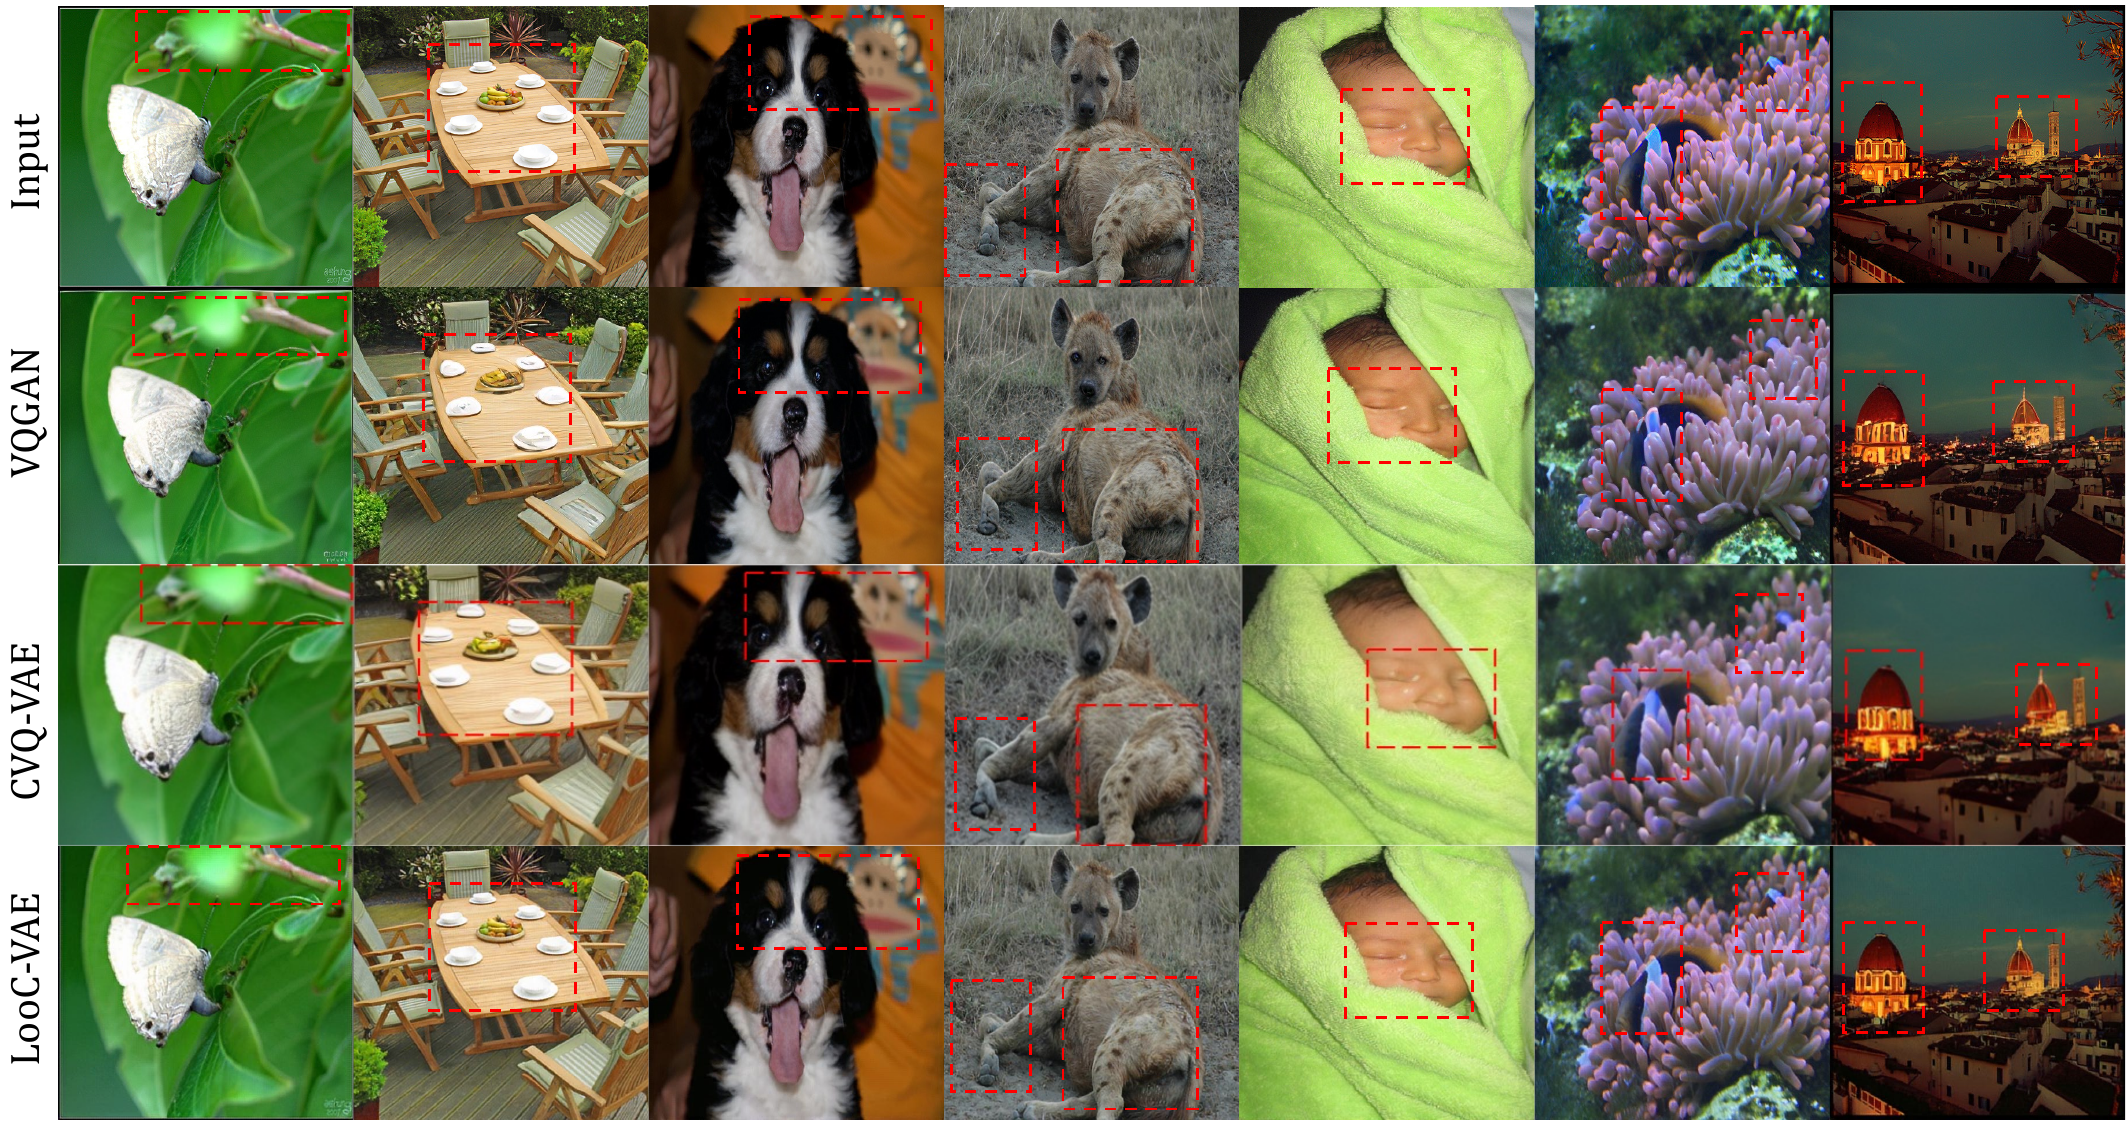}

   \caption{Reconstructions from different models.
      (a)imagenet-valdataion (b)FFHQ-validataion
    }
   \label{supp_fig_reconstruction}
\end{figure*}
