# Supplementary material for: LooC: Effective Low-Dimensional Codebook for Compositional Vector Quantization
Source: arXiv:2601.00222 source file (2026-01-01)
Supplement: Supplementary file 3 [file supp_dim.tex]

% Please add the following required packages to your document preamble:
% \usepackage{multirow}
\begin{table*}[t]
\scalebox{0.75}
{
\begin{tabular}{llllllllllllllllll}
\hline
\multicolumn{1}{c}{\multirow{2}{*}{Method}} & \multicolumn{5}{c}{MNIST(28x28)} & \multicolumn{5}{c}{CIFAR10(32x32)}  &  & \multicolumn{5}{c}{Fashion MNIST(28x28)} \\ \cline{2-6} \cline{8-12} \cline{14-18} 
 & \multicolumn{1}{c}{SSIM} & \multicolumn{1}{c}{LPIPS} & \multicolumn{1}{c}{rFID} & l1 loss & PSNR  &  & \multicolumn{1}{c}{SSIM} & \multicolumn{1}{c}{LPIPS} & \multicolumn{1}{c}{rFID} & l1 loss & PSNR  &  & \multicolumn{1}{c}{SSIM} & \multicolumn{1}{c}{LPIPS} & \multicolumn{1}{c}{rFID} & l1 loss & PSNR  \\ \cline{1-6} \cline{8-12} \cline{14-18} 
Baseline VQ-VAE         & 0.9777 & 0.0282 & 3.43 & 0.0207  & 26.48 &  & 0.8595 & 0.2504 & 39.67 & 0.0527  & 23.32 &  & 0.9140 & 0.0801 & 12.73 & 0.0377  & 23.93 \\
CVQ-VAE                 & 0.9833 & 0.0222 & 1.80 & 0.0180  & 27.87 &  & 0.8978 & 0.1883 & 24.73 & 0.0448  & 24.72 &  & 0.9233 & 0.0693 &  8.85 & 0.0344  & 24.66 \\
Ours dim=2, num=256      &   &    &   &   &    &  &   &    &   &   &    &  &   &    &   &   &    \\
Ours dim=4, num=256      &   &    &   &   &    &  &   &    &   &   &    &  &   &    &   &   &    \\
Ours dim=8, num=256     &   &    &   &   &    &  &   &    &   &   &    &  &   &    &   &   &    \\
Ours dim=16, num=256     &   &    &   &   &    &  &   &    &   &   &    &  &   &    &   &   &    \\
Ours dim=64, num=256     &   &    &   &   &    &  &   &    &   &   &    &  &   &    &   &   &    \\
Ours dim=256, num=256    &   &    &   &   &    &  &   &    &   &   &    &  &   &    &   &   &    \\ \hline
Ours dim=12, num=256    &   &    &   &   &    &  &   &    &   &   &    &  &   &    &   &   &    \\ 
Ours dim=24, num=256    &   &    &   &   &    &  &   &    &   &   &    &  &   &    &   &   &    \\ 
Ours dim=32, num=256    &   &    &   &   &    &  &   &    &   &   &    &  &   &    &   &   &    \\
Ours dim=48, num=256    &   &    &   &   &    &  &   &    &   &   &    &  &   &    &   &   &    \\
Ours dim=128, num=256    &   &    &   &   &    &  &   &    &   &   &    &  &   &    &   &   &    \\ \hline
\end{tabular}
}
\caption{\textbf{Ablation study on various settings.}  Different Dimension of codebook entries.}
%We report pixel-level $l_1$ and PSNR metrics, patch-level SSIM, feature -leavel LPIPS, and dataset-level FID metrics. 
on the validation sets of MNIST, CIFAR10, and Fashion MNIST. Ours is better.
\label{supp_tab_dim}
\end{table*}
